# Supplementary material for: Approaching 100% Confidence in Stream Summary through ReliableSketch
Source: arXiv:2406.00376 source file (2024-06-01)
Supplement: Supplementary file 1 [file ImplementationAppendix.tex]

\presec
\section{Implementations} \postsec
\label{sec:Implementations:appendix}

\subsection{Implementation on RMT switches}
\label{sec:p4:deploy}
We first briefly describe the architecture of RMT (recofigurable match-action table) switches \cite{??}, then we present the implementation of \aname{} on a typical kind of RMT switch, \ie, Tofino switch \cite{?} in P4 language. 

\subsubsection{Architecture of RMT Switches}
We take Tofino switch, a typical kind of RMT switch as example.
Figure \ref{?} shows the pipeline architecture of Tofino switches.
It mainly consists of three components: an Ingress pipeline, a traffic manager (TM), and an Egress pipeline.
Each incoming packet undergoes these three components in sequence.
Each pipeline consists of a parser, a deparser, and multiple stages, and each of the stage has independent memory resources (\eg, SRAM, TCAM) and computing resources (\eg, SALU, hash units).
In the pipeline, Each incoming packet first undergoes the parser, which extracts packet header from the packet for forwarding logic.
Then, the packet access the stages in sequence.
Finally, the packet undergoes the deparser, which reconstructs the packet with the extracted packet header, and then leaves the pipeline.
The TM forwards each packet that leave the Ingress pipeline to the egress pipeline, and the forwarded packet undergoes another pipeline before leaving the switch.

Such RMT architecture is constrained by its limited accessibility: In each stage, the packet can only access the resources in the stage itself.
In other words, the packet can never access the prior stages again.
Usually, this constraint requires the workflow of algorithms to be unidirectional. 
In order to circumvent this constraint, some prior solutions \cite{?} resubmit, mirror, or recirculate packets to access the prior stages at the cost of pipeline forwarding capacity.

\subsubsection{P4 Implementation}

At a high level, we abstract the implementation of \aname{} as a workflow consisting of several modules.

\ppp{Workflow:}
The workflow consists of a cold filter \cite{coldfilter} module, \aname{} module, and a lock module, and the traffic undergoes them in turn.

\bbb{1) Cold filter module:}
This module consists of several pairs of hash function and array.
%, and each pair of hash function and 8-bit counter array is placed in one stage.
%
For each incoming packet, it find a counter in every array, and increase the values by one.
%
%
% When the value of the hashed counter in the first array reaches $u$, it will further enter the second array, and repeats the same operation as in the first array.
%
%
Only the packet that its counter in each array reaches $u$ can further enter the \aname{} module.

\bbb{2) Lock module:}
This module consists of several pairs of hash function and array.
For each packet enter a layer of \aname{} module, they need to get status of the lock, and then decide how to work in \aname{} module.
Besides, \aname{} module could also mirror a packet back here to lock the bucket.

\bbb{3) \aname{} module:}
This module consists of several pairs of hash function and array.
For each array, we build two registers.
The first consists of 32-bit counters, counting the total number of packets.
The second consists of 64-bit counters, each of which is split into two field, first field is to store the ID, and second field counts the collision number of packets.
For each incoming packet, it gets the status from the lock module, determined by the status, the work of a layer will be divided into two classes:

\bbb{Unlocked}: First, the packet will find a bucket in the first register and increase the value of the total counter.
Second, the packet will find the bucket in the second register, checking whether it needs to change the ID storing in the ID field, and then compare the ID, if different, increase the value of collision field. 
Third, the packet will check whether the collision value reaches threshold of the layer, if so, we mirror the packet to lock the bucket.

\bbb{Locked:}In a locked bucket, packet will only find the bucket in second register, and then check whether the ID is match, increasing the value of collision field if matches, if not, the packet will enter the next layer.

\ppp{Hardware Resources Utilization:}
We show the utilization of different types of hardware resources in Table \ref{table:resource}. We can see that the average usage is less than 25\% across all resources. We implement \aname{} in 9 stages on Tofino switch: 1 stage for cold filter module, 7 stages for three layers of \aname{} module and 1 stage for lock module.

\vspace{-0.2cm}
\begin{table}[H]
\caption{H/W resources used by \aname{}. }
%\vspace{0.05in}
\label{table:resource} 
\vspace{-0.3cm}
\begin{tabular}{|m{0.25\columnwidth}|m{0.16\columnwidth}<{\raggedleft}|m{0.33\columnwidth}<{\raggedleft}|} \hline
\textbf{Resource}   & \textbf{Usage} & \textbf{Percentage} \\ \hline
Hash Bits  & 541 & 10.84\% \\
SRAM  & 138 & 14.37\% \\
Map RAM  & 119 & 20.66\% \\
TCAM  & 0 & 0\% \\
Stateful ALU  & 12 & 25.00\% \\
VLIW Instr  & 23 & 5.99\% \\
Match Xbar  & 109 & 7.10\% \\
\hline
\end{tabular}
\vspace{-0.05in}
\end{table}
