# Supplementary material for: Approaching 100% Confidence in Stream Summary through ReliableSketch
Source: arXiv:2406.00376 source file (2024-06-01)
Supplement: Supplementary file 2 [file appendix.tex]

\section{old-pseudo code}
\label{appendix:pscode}

\begin{algorithm}
	\KwIn{An item $e_i$}
    $\hat{f_i} = B[h(e_i)].count * s(e_i)$\;
	\uIf{$e_{i} \in L_{e_i}$}
	{
		update the frequencies\;
	    \uIf{flag for $e_{i}$ is \textbf{false}}
	    {
	        $B[h(e_i)].count \gets B[h(e_i)].count + s(e_i)$\;
	    }
	}
	\uElseIf {$L_{e_i}$ is not full}
	{
	    insert the item with $<\!e_i,~1,~true\!>$\;
	}
	\Else
	{
	    $B[h(e_i)].count \gets B[h(e_i)].count + s(e_i)$\;
		\uIf {$\hat{f_i}$ is not smaller than the smallest counter in $L_{e_i}$}
		{
	        $L_{e_i}.replace(e_i, \hat{f_i} + 1, false)$\;
	    }
	}
	\Return\;
	\caption{Insertion of \aname{}.}
	\label{alg:technique}
\end{algorithm}

\section{old-implementation}
\label{exp:imp}
We have implemented \aname{} and all other algorithms in C++.
The hash functions are implemented using the 32-bit Bob Hash (obtained from the open-source website \cite{bobhash}) with different initial seeds.

\section{old-datsets}

\label{exp:dat}

\ppp{1) Synthetic Datasets:}
We generate $10$ synthetic datasets that follow the Zipf~\cite{zipf} distribution by using Web Polygraph~\cite{webpoly}, an open-source performance testing tool. Each dataset has 32 million items, and the skewness of datasets varies from 0.3 to 3.0. The length of each item ID is $4$ bytes. 
%In the following experiments, we use the dataset with skewness of 1.5 as the synthetic dataset.
%We generate the synthetic datasets using Web Polygraph~\cite{webpoly}, an open-source performance testing tool. Each dataset has 32 million items, and the length of each item ID is $4$ bytes. 
The synthetic datasets can be used to experiment the influence of the distribution of datasets (skewness varying from 0.3 to 3.0).
We also use the dataset with skewness of 1.5 as the synthetic dataset for experiments on the four applications, because this skewness provides an appropriate difficulty of distinguishing items by frequency.
%The frequency variation of different items is so small that items are hard to distinct When the skewness is under 1.5, While it is totally oppisite when the skewness is above 1.5. %
% Steve: why this one? We should state what happens for other values of skewness. Too easy to criticise for a reviewer...
%steve这个问题，或许可以用distribution的实验说一下？

\ppp{2) IP Trace Dataset:}
The IP Trace Dataset is streams of anonymized IP traces collected in 2016 by CAIDA~\cite{caida}. Each item contains a source IP address ($4$ bytes) and a destination IP address ($4$ bytes), 8 bytes in total.

\ppp{3) Web Page Dataset:}
The Web page dataset is built from a collection of web pages, which were downloaded from the website~\cite{webdocs}.
Each item ($4$ bytes) represents the number of distinct terms in a web page.

\ppp{4) Network Dataset:}
The network dataset contains users' posting history on the stack exchange website~\cite{net_dat}. Each item has three values $u,v,t$, which means user $u$ answered user $v$'s question at time $t$. We use $u$ as the ID.

\section{old-computational platform}
\label{compute}
We conduct all the experiments on a machine with two 6-core processors (12 threads, Intel Xeon CPU E5-2620 @2 GHz) and 64 GB DRAM memory. 
Each processor has three levels of cache memory: one 32KB L1 data caches and one 32KB L1 instruction cache for each core, one 256KB L2 cache for each core, and one 15MB L3 cache shared by all cores.

\section{old-parameter settings}

\subsection{old-Parameter Settings for Finding Frequent Items}
\label{appendix:para:fre}
Let $d$ be the number of cells in the Heavy Part of a bucket. For \aname{}, we set $d=16$.
For other sketches, the parameters are set according to the recommendation of their authors. The memory size ranges from 0.2MB to 1MB. We choose such a small memory for the following two reasons.
\begin{itemize}
    \item When using sketches, it is often desired that they fit in the cache to make them fast enough.
    \item Sketches are often sent across the network, and the small size of sketches can significantly save the bandwidth.
\end{itemize}

\subsection{old-Parameter Settings for Other Applications}
\label{appendix:para:app}

For \aname{}, we set $d=16$, which means there are 16 cells in the Heavy Part.
For other sketches, the parameters are set according to their authors' recommendations.
For finding heavy changes, the memory size ranges from 4MB to 8MB, because FR cannot decode with less memory, and \aname{}\_C only uses $\frac{1}{10}$ the memory of FR and FR+CF.
For finding persistent items, the memory size ranges from 0.2MB to 1MB. Because PIE cannot decode with small amounts of memory, it will use $200$ times more memory as Small-Space and \aname{}\_P.
For finding Super-Spreaders, the memory size ranges from 0.6MB to 1MB, because algorithms on this application often need more memory to remove duplicates. We use the IP Trace dataset to evaluate the performance of other applications because only IP Trace datasets can be used to find Super-Spreaders.

\subsection{old-Parameter Settings for Experiments on Distributions}
\label{appendix:para:dis}

To evaluate the impact of the item distribution, we use the synthetic datasets whose skewness ranges from 0.3 to 3.0.
For \aname{}, we set $d=16$, which means there are 16 cells in the Heavy Part. The memory size ranges from 20KB to 60KB, because such little memory better exposes the difference between different distributions.

\section{old-mathematical analysis}
\label{appendix:math}
\subsection{old-Variance and Error Bound}
\label{subsec:appen:error}
Here, we show the variance and the error bound of our estimation for each item $e_i$. 

\begin{theorem}
	\label{theo:variance}
	Let $e_1, e_2, \cdots, e_n$ be the items inserted to $B[h(e_i)]$. We can get the bound of the variance of our estimation that
	\begin{equation}
	\begin{aligned}
    Var(\hat{f_i}) \leqslant \sum_{e_j \neq e_i} (f_j)^2
    \end{aligned}
    \end{equation}
\end{theorem}

\begin{proof}
If $e_i$ is error-free, then $\hat{f_i} = f_i$. Otherwise, we have$\hat{f_i} = \left(\sum_{e_j \in S_e}f_j\cdot s(e_j)\right)\cdot s(e_i)$, where $S_e$ is the set of the items that are not error-free. According to \ref{subsec:math:unbiased}, $E(\hat{f_i})=f_i$, so we get the variance of $\hat{f_i}$ that 
$Var(\hat{f_i}) = E_{s(e_j)\in \{1,-1\}} \left( \left(\sum_{e_j \in S_e,j\neq i}f_j\cdot s(e_j)\right)\cdot s(e_i)\right)^2
=E_{s(e_j)\in \{1,-1\}}\left(\sum_{e_j \in S_e,j\neq i}f_j\cdot s(e_j)\right)^2$

From the analysis in \ref{subsec:math:unbiased}, we find that $s(e_i)$ and whether $e_i$ is error-free is independent. Thus, the cross terms have the same chance to be $1$ and $-1$, so the expectation of their sum is $0$. Therefore, we have
$Var(\hat{f_i}) 
=E_{s(e_j)\in \{1,-1\}}\left(\sum_{e_j \in S_e, j\neq i} (f_j)^2\right)
\leqslant  \sum_{e_j \neq e_i} (f_j)^2$
\end{proof}

According to the variance, we can derive an error bound for $\left\|f\right\|_2$.

\begin{theorem}
Let $l = \frac{e}{\epsilon^2}$, then
$P\left(\left|\hat{f_i}-f_i\right| \geqslant \epsilon \left\|f\right\|_2 \right) \leqslant \frac{1}{e}$
\label{theo:bound2}
\end{theorem}

\begin{proof}
Based on Chebyshev's theorem, we can get that
$P\left(\left|\hat{f_i}-f_i\right| \geqslant \sqrt{e \sum_{e_j \neq e_i} (f_j)^2}\right) 
\leqslant
\frac{Var(\hat{f_i})}{\left(\sqrt{e \sum_{e_j \neq e_i} (f_j)^2}\right)^2} 
\leqslant \frac{1}{e}$. 

For items in $B[h(e_i)]$, we can have an estimation that
$\sum_{e_j} {(f_j)^2} = \frac{1}{l}(\left\|f\right\|_2)^2$. 
Therefore, we can get\\
$P\left(\left|\hat{f_i}-f_i\right| \geqslant \epsilon \left\|f\right\|_2\right) 
\leqslant 
P\left(\left|\hat{f_i}-f_i\right| \geqslant \epsilon \sqrt{l \cdot \sum_{h(e_j)=h(e_i)} f_j^2}\right)
\leqslant
P\left(\left|\hat{f_i}-f_i\right| \geqslant \sqrt{e \sum_{e_j \neq e_i} f_j^2}\right)
\leqslant \frac{1}{e}$
\end{proof}

We can find that this bound is relatively loose because it also takes effect on the items in the Waving Counter.
However, for items in the Heavy Part, $\sqrt{l \cdot \sum_{e_j \neq e_i} (\Delta_i f_j)^2}$ is often much smaller than $\left\|f\right\|_2$. 

Then we compare the error bound of \aname{} with that of SS and USS.
For SS and USS, we can regard the smallest bin in the data structure as the Waving Counter and the other bins in the data structure as the Heavy Part.
Therefore, we can transform SS and USS to one bucket with a Heavy Part and a Waving Counter.
Similar to \aname{}, the error of SS and USS comes from the period when the items are in the smallest bin.
The comparison of their error is shown below.

\begin{theorem}
Let $\left|\hat{f_i}-f_i\right|_{SS}$ be the error  of item in SS and USS, and $\left|\hat{f_i}-f_i\right|_{WS}$ be the error of item in our \aname{}.
If $f_j$ in our \aname{} is same as $f_j$ in SS and USS, we have
\begin{equation}
\begin{aligned}
\sup\left|\hat{f_i}-f_i\right|_{WS} \leqslant
\sup\left|\hat{f_i}-f_i\right|_{SS}
\end{aligned}
\end{equation}
In other words, the error bound of \aname{} is smaller than that of SS and USS.
(Here we use $sup$ to denote a theoretical upper bound, not necessarily the least upper bound.)
\label{theo:compare}
\end{theorem}

\begin{proof}
For \aname{}, we have
$
\sup\left|\hat{f_i}-f_i\right|_{WS} = 
\left|\sum_{e_j \neq e_i}{f_j\cdot s(e_j)}\right|
$. 
%here $e_j$ denotes item inserted into the Waving Counter.
For SS, we have 
$
\sup\left|\hat{f_i}-f_i\right|_{SS} = 
\left|\sum_{e_j \neq e_i}{f_j}\right|
$.
%where $e_j$ denotes item inserted into the smallest bin. 
\par Though the replacement procedure of USS is different from that of SS, they all increment the smallest bin for each item which is not in the sketch.
Therefore, the expression of the error of USS is the same as that of SS.
If $f_j$ in \aname{} is same as $f_j$ in SS and USS, we can get that
\[
\sup\left|\hat{f_i}-f_i\right|_{WS} = 
\left|\sum_{e_j \neq e_i}{ f_j\cdot s(e_j)}\right|
\leqslant \left|\sum_{e_j \neq e_i}{f_j}\right|
=\sup\left|\hat{f_i}-f_i\right|_{SS}\\
\]
We can find that they are equal only when all $s(e_j)$ is $1$ or all $s(e_j)$ is $-1$.
\end{proof}

Even though $f_j$ may be different, $\left|\sum_{e_j \neq e_i}{f_j\cdot s(e_j)}\right|$ is often smaller than $\left|\sum_{e_j \neq e_i}{f_j}\right|$.
It is because we divide the data stream into $l$ buckets. As a result, each item accesses different buckets and the error is divided.
On the contrary, there is only one Waving Counter in SS and USS, so all unilateral accumulations occur in the same Waving Counter and the estimated frequency is highly overestimated.
In other words, the error of \aname{} is often smaller than that of SS and USS.

According to the comparison, we can derive an error bound of $\left\|f\right\|_1$.

\begin{theorem}
Let $l = \frac{e}{\epsilon}$, we have
\[
P\left(\left|\hat{f_i}-f_i\right| \geqslant \epsilon \left\|f\right\|_1 \right) \leqslant \frac{1}{e}
\]
\label{theo:bound1}
\end{theorem}

\begin{proof}
According to Theorem \ref{theo:compare}, we have\\
\[
\mathbb{E}\left[\left|\hat{f_i}-f_i\right|\right]
=
\mathbb{E}\left[\left|\sum_{e_j \neq e_i}{ f_j\cdot s(e_j)}\right|\right]
\leqslant
\mathbb{E}\left[\left|\sum_{e_j \neq e_i}{ f_j}\right|\right]
\leqslant
\frac{\epsilon \left\|f\right\|_1}{e}
\]

By the Markov inequality,
\[
P\left(\left|\hat{f_i}-f_i\right| \geqslant \epsilon \left\|f\right\|_1 \right)
\leqslant 
P\left(\left|\hat{f_i}-f_i\right| \geqslant e \mathbb{E}\left[\left|\hat{f_i}-f_i\right|\right]\right)
\leqslant
\frac{1}{e}
\]  
\end{proof}

% \begin{theorem}
% Assume that $n$ is the number of different items inserted into the waving counter of $B[h(e_i)]$ and $f_1\geq f_2\geq \cdot\cdot\cdot\geq f_n$ is the frequency of the $n$ items that is not error-free. With probability $2\phi(\lambda) - 1$,
% \begin{equation}
% \begin{aligned}
% \left|\hat{f_i}-f_i\right|\leqslant \sum_{k=1}^{l}f_k-\sum_{k=l+1}^{n}f_k
% \end{aligned}
% \end{equation}
% where $\phi(x)$ is the Cumulative distribution function for normal distribution $N(0,1)$, $l = \frac{[\lambda \sqrt{n}]+n}{2}$, 
% $[x]=\max\{y \in \mathbb{Z}:y\leqslant x\}$.
% \end{theorem}

% \begin{proof}
% $s(e_j)$ are independent and identical distributions, which satisfy 
% \[
% E(s(e_j)) = 0,Var(s(e_j)) = 1
% \]

% According to the central limit theorem, 
% \[
% {\lim_{n \to +\infty}}P(-\lambda\leqslant\frac{\sum_ {k=1}^{n}s(e_k)}{\sqrt{n}}\leqslant\lambda) =2\phi(\lambda) - 1
% \]
% So with probability $2\phi(\lambda) - 1$, the number of items with the same $s(e_i)$ is less than $\frac{[\lambda \sqrt{n}]+n}{2}$. Thus,
% \begin{equation}
% \begin{aligned}
% \left|\hat{f_i}-f_i\right|
% &=\sum_{e_j \neq e_i}{f_j\cdot s(e_j)}\cdot s(e_i)
% \leqslant\left|\sum_ {k=1}^{n}s(e_k)\cdot f_k\right|\\
% &\leqslant\sum_{k=1}^{l}f_k-\sum_{k=l+1}^{n}f_k
% \end{aligned}
% \end{equation}
% \end{proof}

\subsection{old-Parameter Analysis}
\label{subsec:appen:para}
We analyze the influence of parameters in \aname{}.
We use $c = dl$ to denote the number of cells in \aname{}.
%We can find that $c = dl$.
Then we show that for fixed $c$, how $d$ influences the performance of our \aname{}.

\begin{theorem}
Let $e_i$ be the $i_{th}$ most frequent item in the data stream. The probability that its frequency $f_i$ is among top-$d$ largest frequencies in bucket $B[h(e_i)]$ is at least
$
1 - \frac{d^d}{d!}\cdot \left(\frac{i-1}{c}\right)^{d}
$
\end{theorem}

\begin{proof}
Let $P_{i}$ be the probability that $B[h(e_i)]$ contains at least $d$ items whose frequency is higher than $e_i$. 
When $i \leqslant d$, $P_{i} = 0$.
So we only need to discuss the case that $i > d$.
When $i > d$, we have
$P_{i}
    \leqslant \dbinom{i-1}{d}\cdot\left(\frac{1}{l}\right)^{d} \leqslant \frac{d^d}{d!}\cdot \left(\frac{i-1}{c}\right)^{d}$. 
Therefore, the probability that $f_i$ is among top-$d$ largest frequencies in bucket $B[h(e_i)]$ is at least
$
1 - \frac{d^d}{d!}\cdot \left(\frac{i-1}{c}\right)^{d}
$.
\end{proof}
We can find that, when $i$ decreases, $P_i$ decreases sharply, which indicates that the probability that $e_i$ is top-$d$ items in $B[h(e_i)]$ becomes much higher.
According to Stirling's approximation,
\begin{equation}
\begin{aligned}
1 - \frac{d^d}{d!}\cdot \left(\frac{i-1}{c}\right)^{d}
\approx 
1 - \frac{1}{\sqrt{2 \pi d}} \cdot \left(\frac{e (i - 1)}{c}\right)^{d}
\end{aligned}
\end{equation}
\par We can also find that, when $i < \frac{c}{e} + 1$, the probability that  $e_i$ is top-$d$ items in $B[h(e_i)]$ increases with $d$ increasing.
