# Supplementary material for: Approaching 100% Confidence in Stream Summary through ReliableSketch
Source: arXiv:2406.00376 source file (2024-06-01)
Supplement: Supplementary file 4 [file 9NetworkAppendix.tex]

\input{vldb/Experiment/sim.tex}
\input{vldb/Experiment/testbed.tex}

\begin{table}[H]
\caption{Time Consumption of Aggregation.}
%\vspace{0.05in}
\label{table:time} 
\vspace{-0.3cm}
\begin{tabular}{m{0.21\columnwidth}<{\centering}|m{0.21\columnwidth}<{\centering}|m{0.21\columnwidth}<{\centering}|m{0.21\columnwidth}<{\centering}}
\bottomrule[1pt]
% \hline
\textbf{Total}   & \textbf{Sync.} & \textbf{Collection} & \textbf{Analysis} \\ \hline
$1.005\ sec$ & $995.566\ msec$ & $3.612\ msec$ & $5.387\ msec$ \\
% \hline
\toprule[1pt]
\end{tabular}
\vspace{-0.05in}
\end{table}

\ppp{Network-wide aggregation mechanism:}
We have also implemented a set of aggregations mechanism for collecting data structures on each switch in the whole network.
The mechanism includes some \texttt{sender} agents and an \texttt{aggregator} agent.
The \texttt{sender} runs on the control plane of each switch deployed with \aname{}, periodically synchronizes the data of the \aname{} from the data plane, and sends the synchronized \aname{} to the \texttt{aggregator}.
The \texttt{aggregator} runs on a server, collects the \aname{}es sent by all switches, and performs data analysis.
Table \ref{table:time} lists the time consumption of each part of the aggregation process.

\input{vldb/Body/ExtensionsAppendix}
\input{vldb/Body/applivationV2}
