# Supplementary material for: Approaching 100% Confidence in Stream Summary through ReliableSketch
Source: arXiv:2406.00376 source file (2024-06-01)
Supplement: Supplementary file 5 [file ExtensionsAppendix.tex]

\presec
\section{Extensions}\postsec{}
\label{sec:extensions:appendix}


\subsection{Network-wide Deployment}

In a network, \anamelong{} can be deployed on user specified switches to measure the traffic. On the one hand, the accuracy can be improved by multiple sketches. On the other hand, we can find abnormal flow size changes without false positives.

\ppp{Accuracy improvement by multiple sketches.}
When a flow passes through multiple sketches on multiple switches, we can query its flow size in these sketches. Each sketch reports a possible flow size interval, \ie, $[\widehat{f_e}-MPE, \widehat{f_e}]$. The intersection of these intervals is a more accurate answer.

\ppp{Anomaly detection.} When a same flow passes through two sketches and they report two flow size intervals without intersection, we know that the flow size must have changed, without false positive.
In this case, we report potential packet drops if the flow size decreased, and report potential loops if the flow size increased.
More details are in \cref{sec:extensions:appendix:packetdrop}.


\subsection{The Mice Flow Filter}
\label{sec:extensions:appendix:micefilter}
We detail the mice filter in this section.
The first layer of \anamelong{} is the largest layer and it takes more than $50\%$ space of the whole \anamelong{}. 
But the first layer is inefficient when mice flows takes a large portion in the traffic. Because the mice flows will increment the NO counters sharply and lock most buckets in the first layers. In this case, many buckets are wasted to record the mice flows. 

Specifically, inspired by CU \cite{estan2002cusketch}, the filter consists of two arrays ($F_1[]$ and $F_2[]$) and each array has $\frac{1}{2} w_1$ $L$-bit counters. For every flow ID $e$, we use two hash functions $h_1^{(1)}(.)$ and $h_1^{(2)}(.)$ to select two mapped counters $C_1=F_1[h_1^{(1)}(e)]$ and $C_2=F_1[h_1^{(1)}(e)]$. To insert a packet with flow ID $e$, if 
any of its two mapped counters is less than $\lambda_1$, we regard it as a mice flow. For a mice flow, we drop it and increment the minimal mapped counter(s) less than $\lambda_1$ by one. Otherwise, when both mapped counters equal to $\lambda_1$, we regard it as a non-mice flow, and pass the packet to the second layer.

In practice, 8-bit counters are sufficient for the filter. Compared to a layer composed of 72-bit error-sensible buckets, the filter can reduce the space cost of layer-1 nearly $10$ times while incurring small controllable errors. The overall accuracy will be significantly improved when we move the space saved by the filter to the other layers. But we cannot replace other layers by the filter because the filter cannot estimate elephant flows well.

% But the first layer is inefficient when mice flows takes a large portion in the traffic. Because the mice flows will increment the NO counters sharply and lock most buckets in the first layers. In this case, many buckets are wasted to record the mice flows. 

% The first layer of \anamelong{} is the largest layer and it takes more than $50\%$ space of the whole \anamelong{}. 
% But the first layer is inefficient when mice flows takes a large portion in the traffic. Because the mice flows will increment the NO counters sharply and lock most buckets in the first layers. In this case, many buckets are wasted to record the mice flows. 



\begin{figure}[htbp]
    % \prefig
    \centering  
    \includegraphics[width=0.96\linewidth]{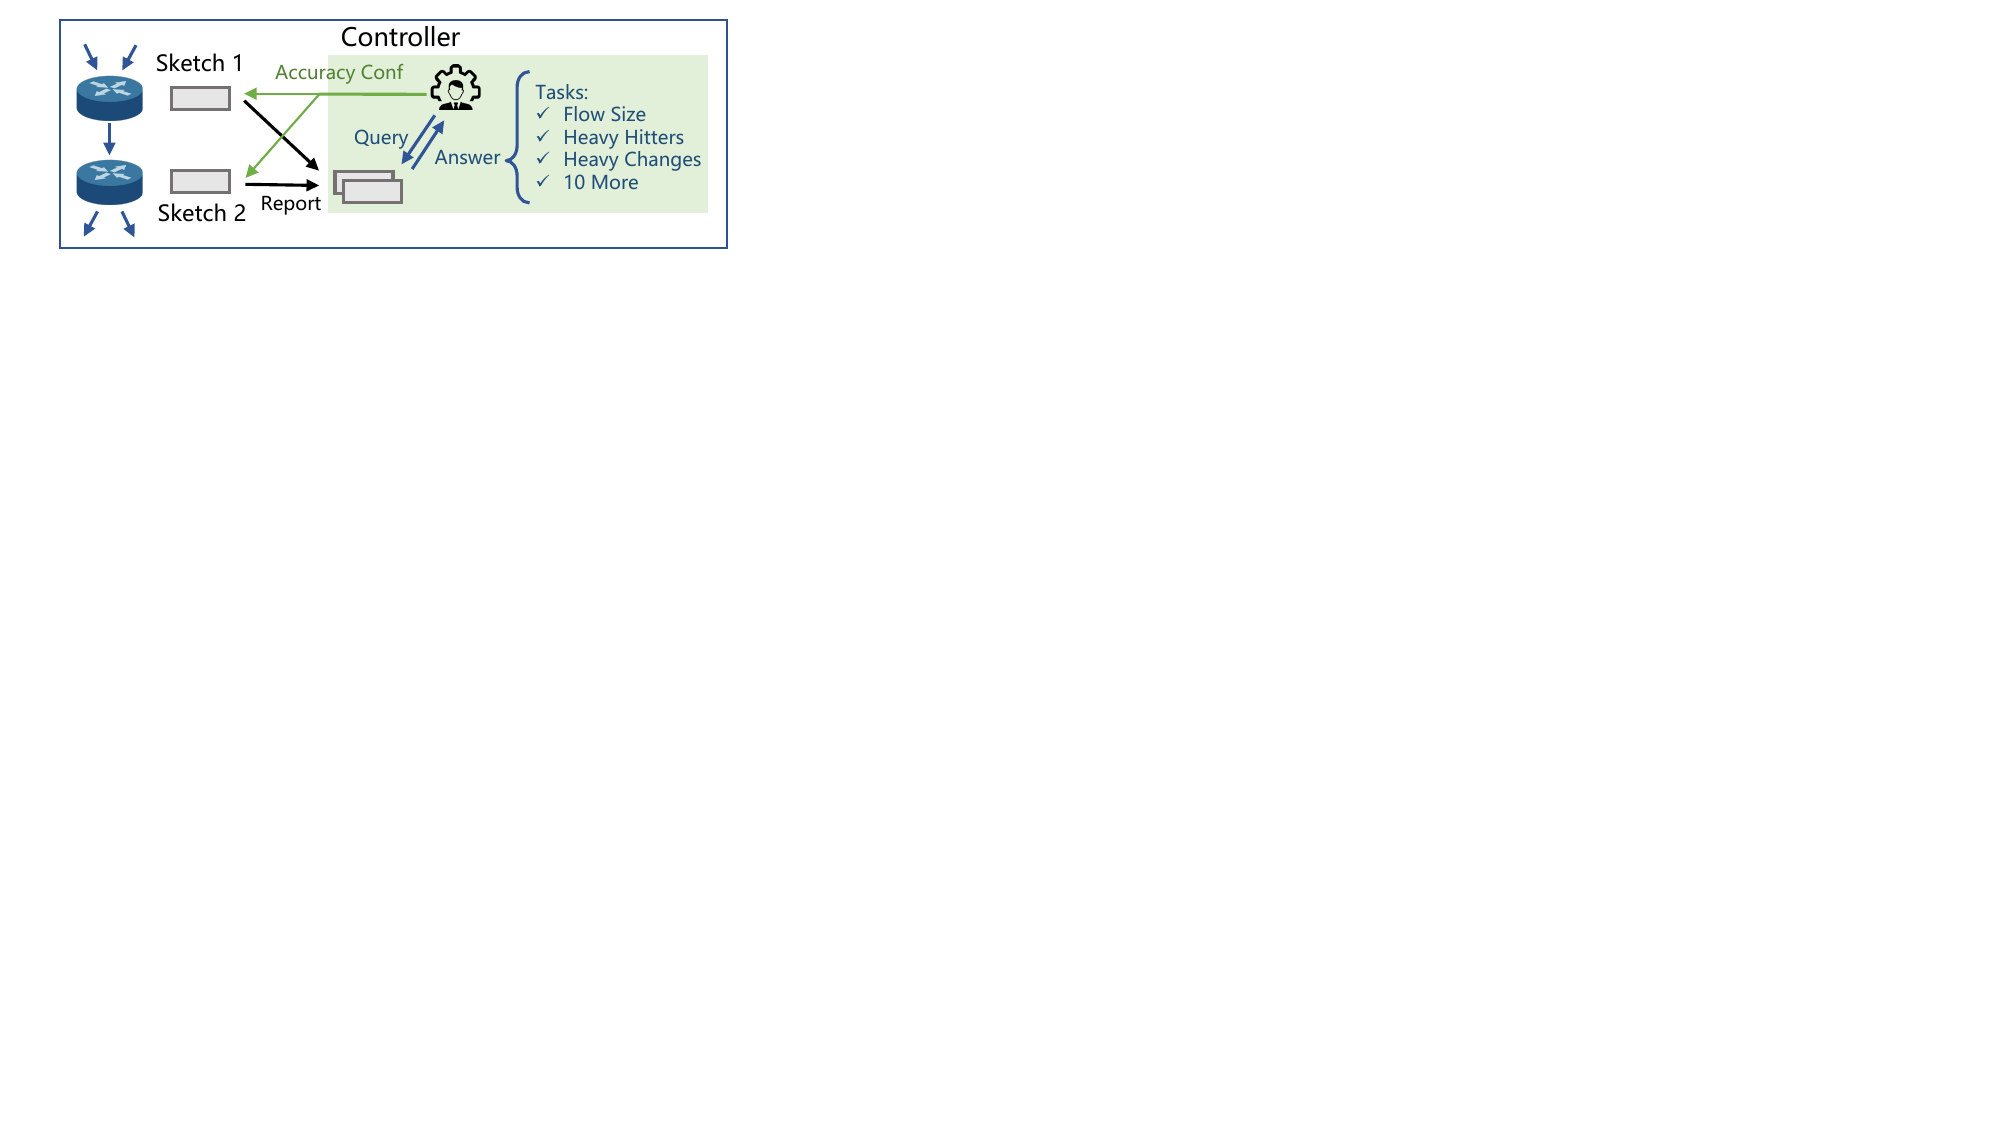}
    \vspace{-0.15in}
    \caption{Sketch Deployment.}
    \label{sketch}
    \postfig
\end{figure}

\presub
\subsection{Detecting Packet Drops and Heavy Changes} \postsub
\label{sec:extensions:appendix:packetdrop}

To detect packet drop in a link, we deploy two \aname{}es $S_1, S_2$ in the up-link switch and down-link switch respectively. 
In each time period, each sketch count all passing packets. At the end of the time period, each sketch is read from the data plane to the control plane and sent to the controller.
The controller scan the two sketches. For each recorded flow, the controller estimates its flow size interval in the two sketches respectively.
If the intersection of the two flow size intervals is empty, the number of packets passing through the upstream switch and the downstream switch must be different. We know that the flow is abnormal and alarm it.

\ppp{Accuracy:} 
All packet loss reports can ensure that the number of packets must have changed, and there will be no false alarm due to sketch errors.
Suppose that the two \aname{}es $S_1, S_2$ are with error thresholds $\Lambda_1$ and $\Lambda_2$. A flow with at least $\Lambda_1+\Lambda_2$ lost packets much trigger the alarm.


\ppp{Detecting Heavy Changes:} 
The heavy changes are flows whose frequency changes in adjacent time windows exceeds $T$. 
To detect heavy changes, the controller saves the sketch in the last period and compare it with the new sketch. Similar to the packet drop, we can find all flows whose frequency changes are no less that $\Lambda_1+\Lambda_2$.
