# Supplementary material for: Approaching 100% Confidence in Stream Summary through ReliableSketch
Source: arXiv:2406.00376 source file (2024-06-01)
Supplement: Supplementary file 6 [file appendixV2.tex]

{\centering \section*{APPENDIX}}


\input{vldb/Body/math_appendix}
\input{vldb/Body/ExtensionsAppendix}
% \input{vldb/Body/ImplementationAppendix}
\input{vldb/Body/applivationV2}
\input{vldb/Body/exp_app}
